# Supplementary material for: On the resistance minimum in LaAlO$_3$/Eu$_{1-x}$La$_x$TiO$_3$/SrTiO$_3$ heterostructures
Source: arXiv:2109.00620 ancillary file (2021-09-01)
Supplement: Supplementary file 1 [file ETO_Supplement.pdf]

# Supplementary Information for On the resistance minimum in $LaAlO_3/Eu_{1-x}La_xTiO_3/SrTiO_3$ heterostructures

N. Lebedev,[1] Y. Huang,[2] A. Rana,[3,4] N. Gauquelin,[5] J. Verbeeck,[5] and J. Aarts[1]

[1] *Kamerlingh Onnes Laboratory, Leiden University, P.O. Box 9504, 2300 RA Leiden, The Netherlands*

[2] *Van der Waals-Zeeman Institute, University of Amsterdam, Science Park 904, 1098 XH Amsterdam, The Netherlands*

[3] *Center for Advanced Materials and Devices, BML Munjal University (Hero Group), Gurgaon, India - 122413*

[4] *MESA+ Institute for Nanotechnology, University of Twente, P.O. Box 217, 7500 AE Enschede, The Netherlands*

[5] *Electron Microscopy for Materials Science, University of Antwerp, Campus Groenenborger Groenenborgerlaan 171, 2020 Antwerpen, Belgium*

(Dated: September 1, 2021)

## I. ADDITIONAL AFM, RHEED AND HAADF DATA

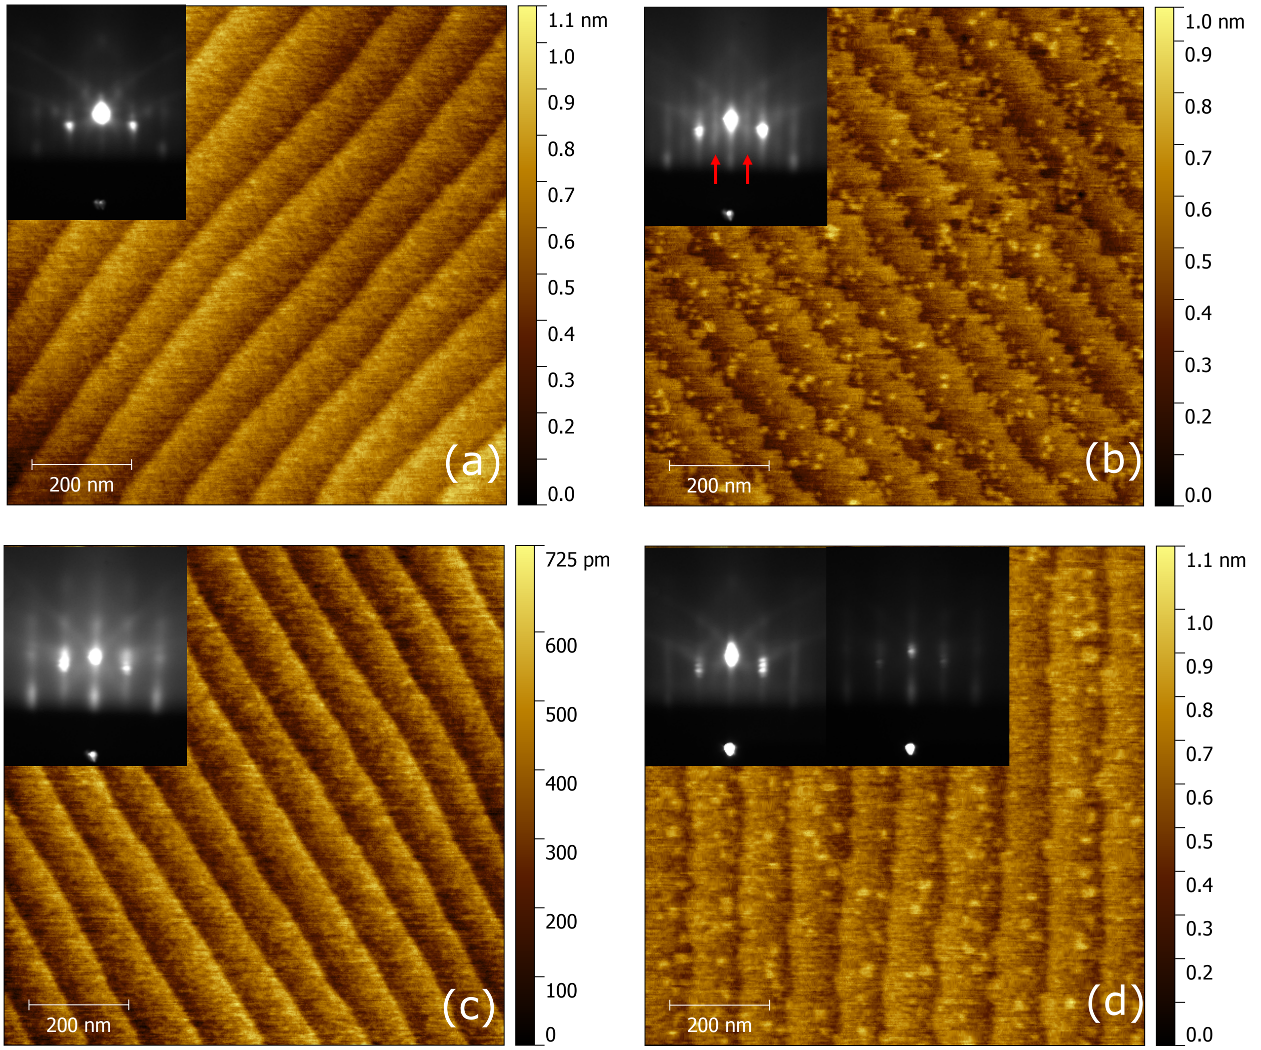


FIG. S1. (a)-(d) AFM images of the surfaces of $TiO_2$-terminated STO, ETO(4 u.c.)/STO, LAO/STO and LAO/ELTO(2 u.c.)/STO, respectively. The insets show the corresponding RHEED patterns after deposition. Red arrows are guides to the eye. In the inset of (d), the left RHEED pattern was taken after deposition of ELTO, the right one after deposition of LAO.

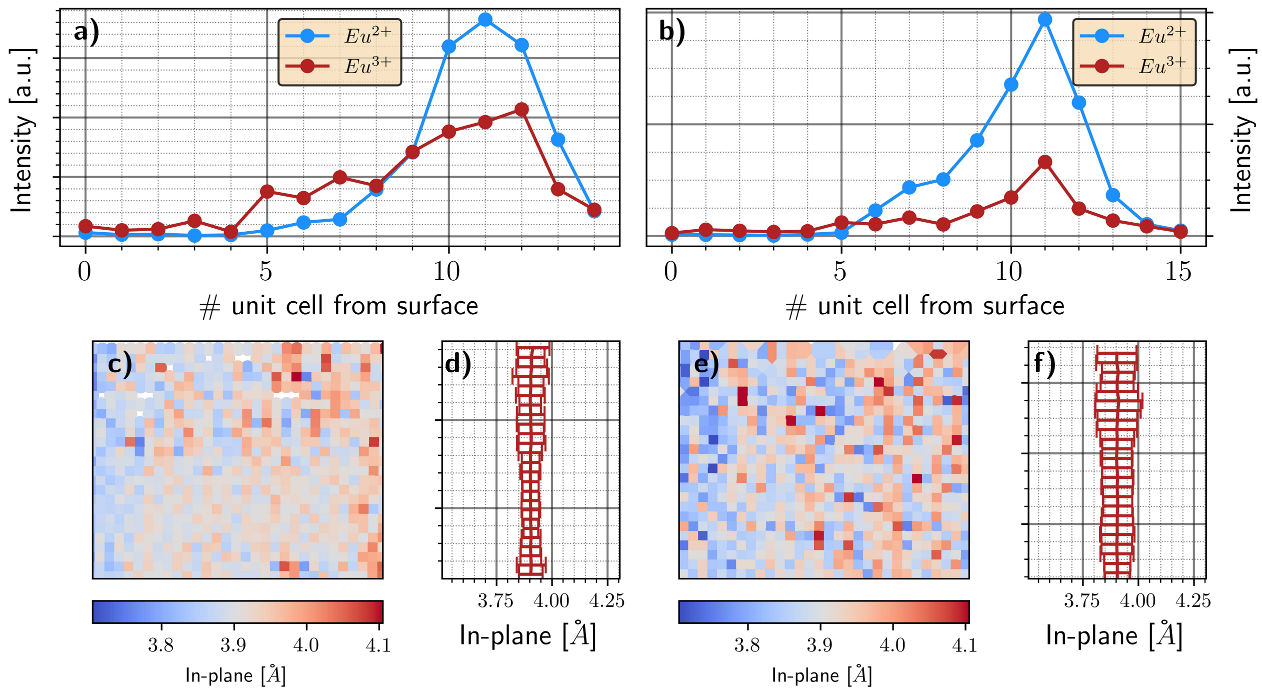


FIG. S2. EELS analysis of the occurrence of $Eu^{2+}$ and $Eu^{3+}$ as function of unit cell distance from the surface for (a) LAO/ETO/STO and (b) LAO/ELTO/STO. (c)-(d) Analysis of the in-plane lattice parameters in LAO/ETO/STO from the image in Fig. 2c in the main text. (e)-(f) the same for LAO/ELTO/STO.

## II. TEMPERATURE DEPENDENCE OF MR AND AHE ANALYSIS

In LAO/STO, the value of the MR as function of an applied magnetic field out of the plane of the sample continuously increases with decreasing temperature (Fig. S3a). The high values of MR, around 50 %, and the almost linear shape in high fields below 50 K point to spatial conductance fluctuation (see Ref. 1–8). In the doped samples, the MR behavior is less monotonous; The MR increased only up to 10-12% until the temperature reaches 10 K (Fig. S3b,c). Below that temperature, the MR decreases, tracing the upturn in the temperature dependence of $R_S$.

To analyze the data with respect to carrier densities $n_i$ and mobilities $\mu_i$ in the presence of AHE, we followed the subtraction method described in Ref. 9. To increase the precision of the fit, we used the derivative of the subtraction result to determine the fitting range. The two-band analysis in a regime without AHE was performed using the fitting of the

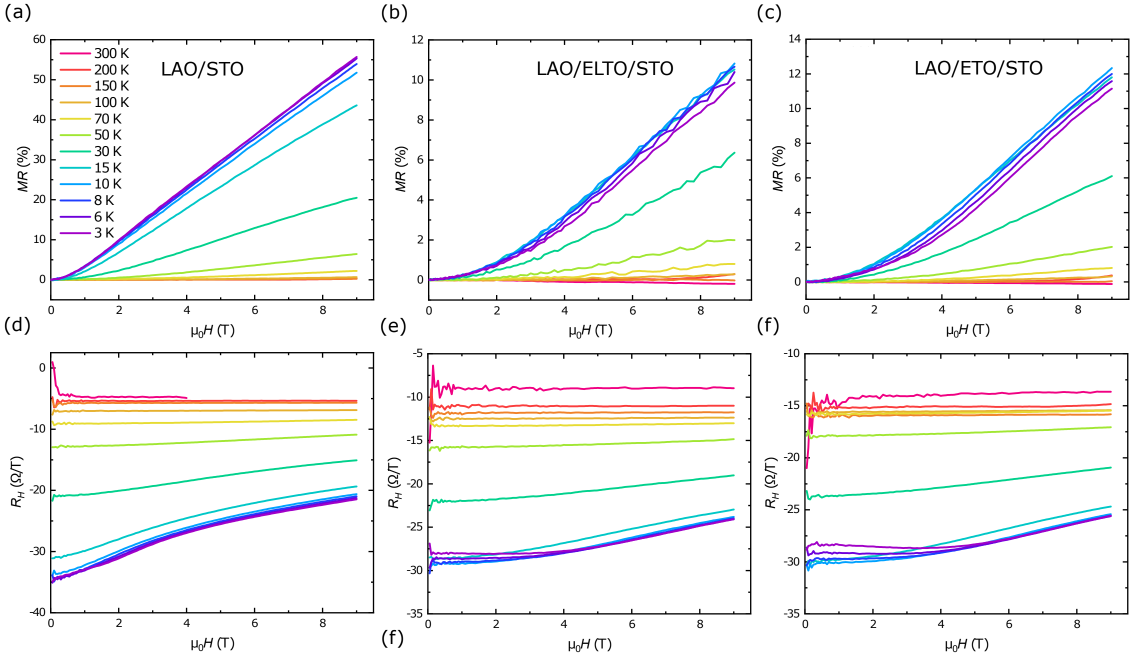


FIG. S3. Magnetoresistance MR at different temperatures indicated by the colors for (a) LAO/STO, (b) LAO/ETO/STO, and (c) LAO/ELTO/STO . The Hall coefficient at different temperatures (same colors as in a,b,c) for (d) LAO/STO, (e) LAO/ETO/STO, and (f) LAO/ETO/STO.

conductance tensor components (see for instance Ref. 10).

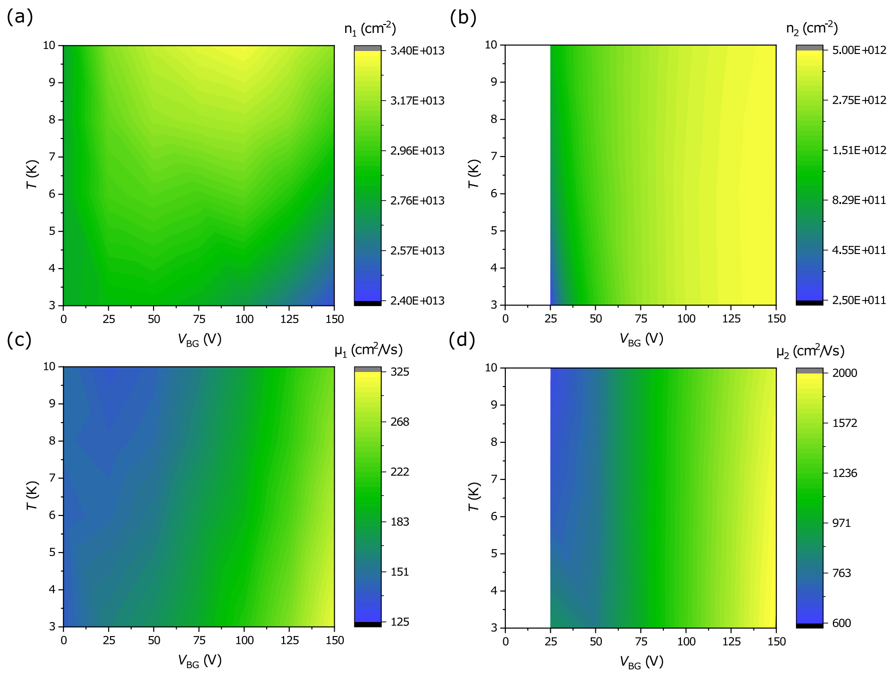


FIG. S4. Temperature and back gate voltage dependence of (a-b) carrier concentrations and (c-d) mobilities for the LAO/ELTO/STO sample. The color scale for all quantities gives the range of their values.

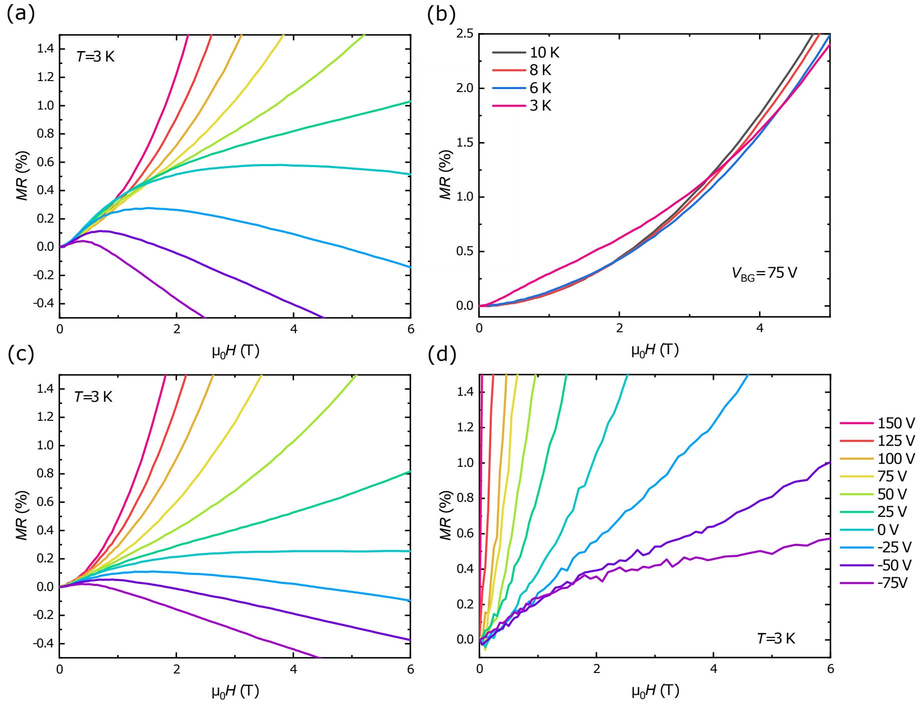


FIG. S5. (a) Magnetoresistance MR with the field out of the plane for LAO/ETO/STO at 3 K. (b) MR for LAO/ETO/STO at $V_{BG} = 75\ V$. Magnetoresistance MR with the field out of the plane at various back gate voltages as indicated for (c) the LAO/ELTO/STO sample and (d) the LAO/STO sample at 3 K. The legend for panels (a) and (b) is the same as in (d).

## III. BACK GATE DEPENDENCE OF THE AHE

In STO-based interfaces, the AHE is often attributed to skew scattering[11,12], one of the extrinsic mechanism for the AHE[13–15], in this case in the second band[11,12]. To shed more light on the mechanism responsible for the AHE, we performed a scaling analysis of the conductivity by calculating the values for $\sigma_{xx}$ and $\sigma_{xy}$, as follows[16]:

$$\sigma_{xx} = \frac{R_S}{R_S^2 + R_{xy}^{AHE\,2}}, \quad \sigma_{xy} = \frac{R_{xy}^{AHE}}{R_S^2 + R_{xy}^{AHE\,2}}, \tag{1}$$

and then plotting them against each other. The results are shown in Fig. S6a for 3 K and in Fig. S6b, for all temperatures. We observe that $\sigma_{xy}$ scales with $\sigma_{xx}$ as $\sigma_{xy} \approx \sigma_{xy}^{1.8-2}$ in the region $\sigma_{xx} > 10^{-3}\ \Omega^{-1}m^{-1}$. This exponent is close to the value of 1.6 observed in the scaling of ELTO metal films[16], which is often attributed to the intrinsic contribution to the AHE, suppressed by the disorder. Nevertheless, the meaning of scaling is somewhat limited because it corresponds to the region, where $R_{xy}^{AHE}$ changes less significantly than the decrease of the sheet resistance.

A final note concerns the behavior of the fitting parameter $M_{eff}$ in the extraction of $R_{xy}^{AHE}$. As seen in Fig. S7a,c, it shows enhancement in regions where the AHE vanishes, for instance at temperatures above 8 K and in the gate voltage range below 25 V. Most likely, the hyperbolic tangent function becomes inadequate to describe the almost flat curve. Furthermore, in most of $V_{BG} - T$ space, the ratio $M_{eff}/T$ is only weakly temperature-dependent (Fig. S7b,d). Still, the point to keep in mind is that we observe the AHE in the temperature-voltage regime where the earlier studies found magnetism. A better way to establish the behavior of magnetization could be the study of the temperature dependence of the ratio $R_{xy}^{AHE}/R_{xy}^{AHE}$(3 K) because it is proportional to the temperature dependence of $M_S/M_S(3K)$ as long as carrier concentration and mobilities do not change significantly. In Fig. S6c, we plot $R_{xy}^{AHE}/R_{xy}^{AHE}$(3 K) at gate voltages above Lifshitz point. The ratio increases with temperature, but we do not see saturation as in Ref. 17 (note that the way in which $R_{xy}^{AHE}$ is extracted in Ref. 17, by simple linear extrapolation, is different from ours). The temperature dependence of $R_{xy}^{AHE}/R_{xy}^{AHE}$(3 K) changes from linear at 25 V to upward curving at higher voltages. Still, as it shows a clear increase from roughly 0, it can be a signature of ferromagnetic behavior.

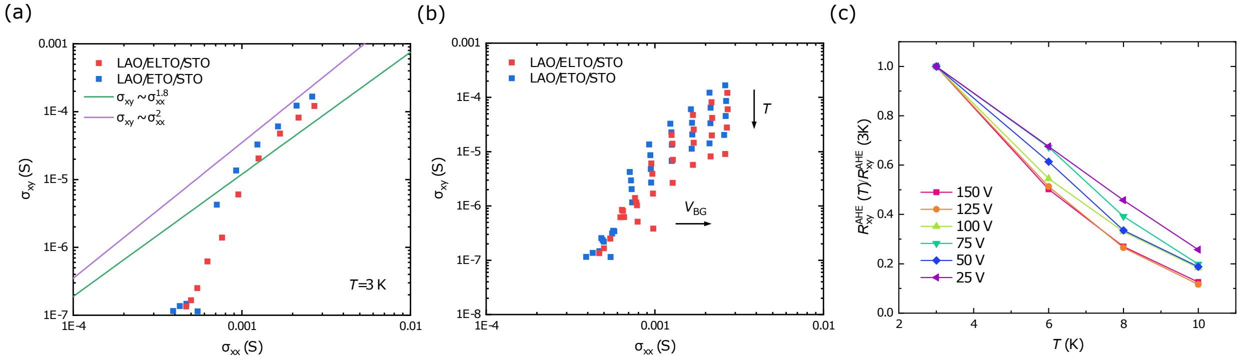


FIG. S6. (a) A plot of the conductances $\sigma_{xy}$ versus $\sigma_{xx}$ at 3 K to investigate Scaling behavior. (b) Plot of $\sigma_x$ versus $\sigma_{xx}$ in order to analyze conductance scaling. Note that trend of a decrease of $\sigma_{xy}$ with increasing temperature is followed poorly in the region $\sigma_{xx} < 8 \times 10^{-4}\Omega^{-1}$ m$^{-1}$. (c) Temperature and back gate voltage dependence of the normalized Anomalous Hall coefficient $R_{xy}^{AHE}$ for the LAO/ELTO/STO sample.

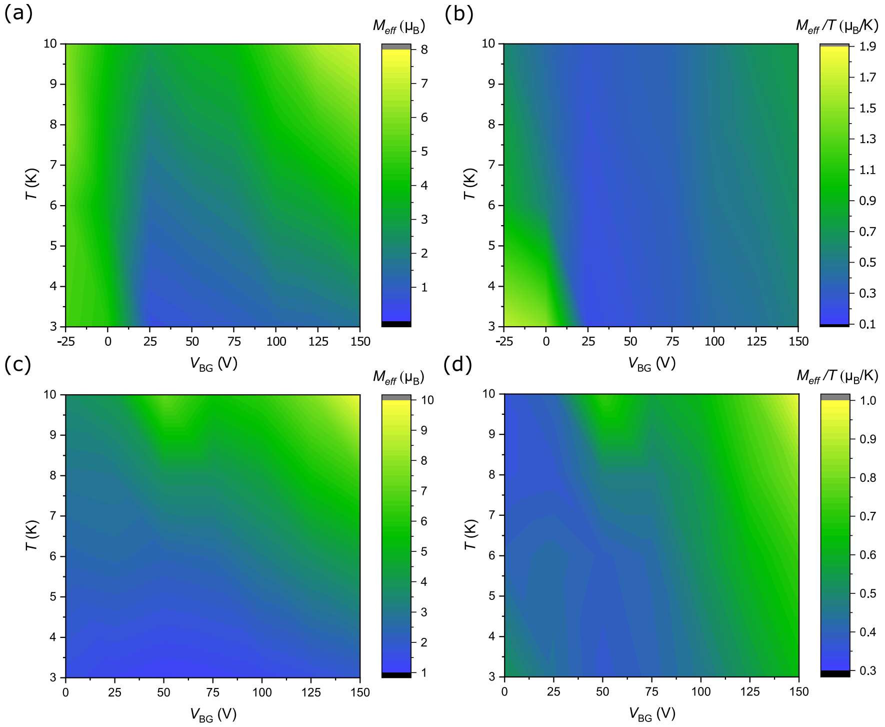


FIG. S7. Temperature and back gate voltage dependence of the fit parameter $M_{eff}$ for (a-b) the LAO/ETO/STO sample and (c-d) the LAO/ELTO/STO sample.

[1] M. M. Parish and P. B. Littlewood, Nature **426**, 162 (2003).

[2] T. Khouri, U. Zeitler, C. Reichl, W. Wegscheider, N. E. Hussey, S. Wiedmann, and J. C. Maan, Phys. Rev. Lett. **117**, 256601 (2016).

[3] J. Hu, M. M. Parish, and T. F. Rosenbaum, Phys. Rev. B **75**, 214203 (2007).

[4] F. Kisslinger, C. Ott, and H. B. Weber, Phys. Rev. B **95**, 024204 (2017).

[5] N. Ramakrishnan, Y. T. Lai, S. Lara, M. M. Parish, and S. Adam, Phys. Rev. B **96**, 224203 (2017).

[6] T. Schumann, M. Goyal, D. A. Kealhofer, and S. Stemmer, Phys. Rev. B **95**, 241113 (2017).

[7] J. Xu, M. K. Ma, M. Sultanov, Z.-L. Xiao, Y.-L. Wang, D. Jin, Y.-Y. Lyu, W. Zhang, L. N. Pfeiffer, K. W. West, K. W. Baldwin, M. Shayegan, and W.-K. Kwok, Nature Communications **10**, 287 (2019).

[8] N. Lebedev, M. Stehno, A. Rana, N. Gauquelin, J. Verbeeck, A. Brinkman, and J. Aarts, Journal of Physics: Condensed Matter **33**, 055001 (2020).

[9] N. Lebedev, M. Stehno, A. Rana, P. Reith, N. Gauquelin, J. Verbeeck, H. Hilgenkamp, A. Brinkman, and J. Aarts, Scientific Reports **11**, 10726 (2021).

[10] A. E. M. Smink, J. C. de Boer, M. P. Stehno, A. Brinkman, W. G. van der Wiel, and H. Hilgenkamp, Phys. Rev. Lett. **118**, 106401 (2017).

[11] A. Joshua, J. Ruhman, S. Pecker, E. Altman, and S. Ilani, Proceedings of the National Academy of Sciences **110**, 9633 (2013).

[12] F. Gunkel, C. Bell, H. Inoue, B. Kim, A. G. Swartz, T. A. Merz, Y. Hikita, S. Harashima, H. K. Sato, M. Minohara, S. Hoffmann-Eifert, R. Dittmann, and H. Y. Hwang, Phys. Rev. X **6**, 031035 (2016).

[13] J. Smit, Physica **21**, 877 (1955).

[14] J. Smit, Physica **24**, 39 (1958).

[15] N. Nagaosa, J. Sinova, S. Onoda, A. H. MacDonald, and N. P. Ong, Rev. Mod. Phys. **82**, 1539 (2010).

[16] K. S. Takahashi, H. Ishizuka, T. Murata, Q. Y. Wang, Y. Tokura, N. Nagaosa, and M. Kawasaki, Science Advances **4** (2018), 10.1126/sciadv.aar7880.

[17] D. Stornaiuolo, C. Cantoni, G. M. De Luca, R. Di Capua, E. Di. Gennaro, G. Ghiringhelli,

B. Jouault, D. Marrè, D. Massarotti, F. Miletto Granozio, I. Pallecchi, C. Piamonteze, S. Rusponi, F. Tafuri, and M. Salluzzo, Nature Materials **15**, 278 (2015).
